# Supplementary material for: 3D Gaussian Editing with A Single Image
Source: arXiv:2408.07540 source file (2024-08-14)
Supplement: Supplementary file 1 [file X_suppl.tex]

% 补充材料
% 1. 证明平移、旋转、放缩的细节

% Appendix
% \appendix

% \newpage

\section{Implementation Details}

All experiments are performed on a PC with an NVIDIA RTX 3090 GPU with 24GB memory. We leverage Adam optimizer\cite{adam} using default parameters of $\alpha=0.02, \beta_1=0.9$ and $\beta_2=0.999$ and use the same learning rate as the original 3D GS\cite{3dgs} for the Gaussian parameters, with a cosine scheduler to interpolate the learning rate of means.

\subsection{Anchor Initialization}

The number of anchor points has a great impact on the optimization process. Too few anchor points limit the freedom of deformation, thus hindering the alignment with the reference image. Too many anchor points restrain the gradient from effective propagation through the occluded object parts, thus slowing down the convergence. Therefore, we choose to select a different number of anchor points based on the geometric complexity of the scene. For all characters in the 3DBiCar\cite{3dbicar}, we sample 800 anchor points. For the NS dataset, we sample different numbers according to editing operations, such as 3000 anchor points for Lego deformation and 800 anchor points for Chair stretching. To explore the influence of the number of anchor points, we compare the optimization results of the coarse stage under different numbers of anchor points in Fig.~\ref{fig:anchor}. Noticeably, as the number of anchor points increases, the rendered image aligns better with the reference image, while too many anchors lead to structural instability.

\begin{figure}
    \centering
    \includegraphics[width=0.99\linewidth]{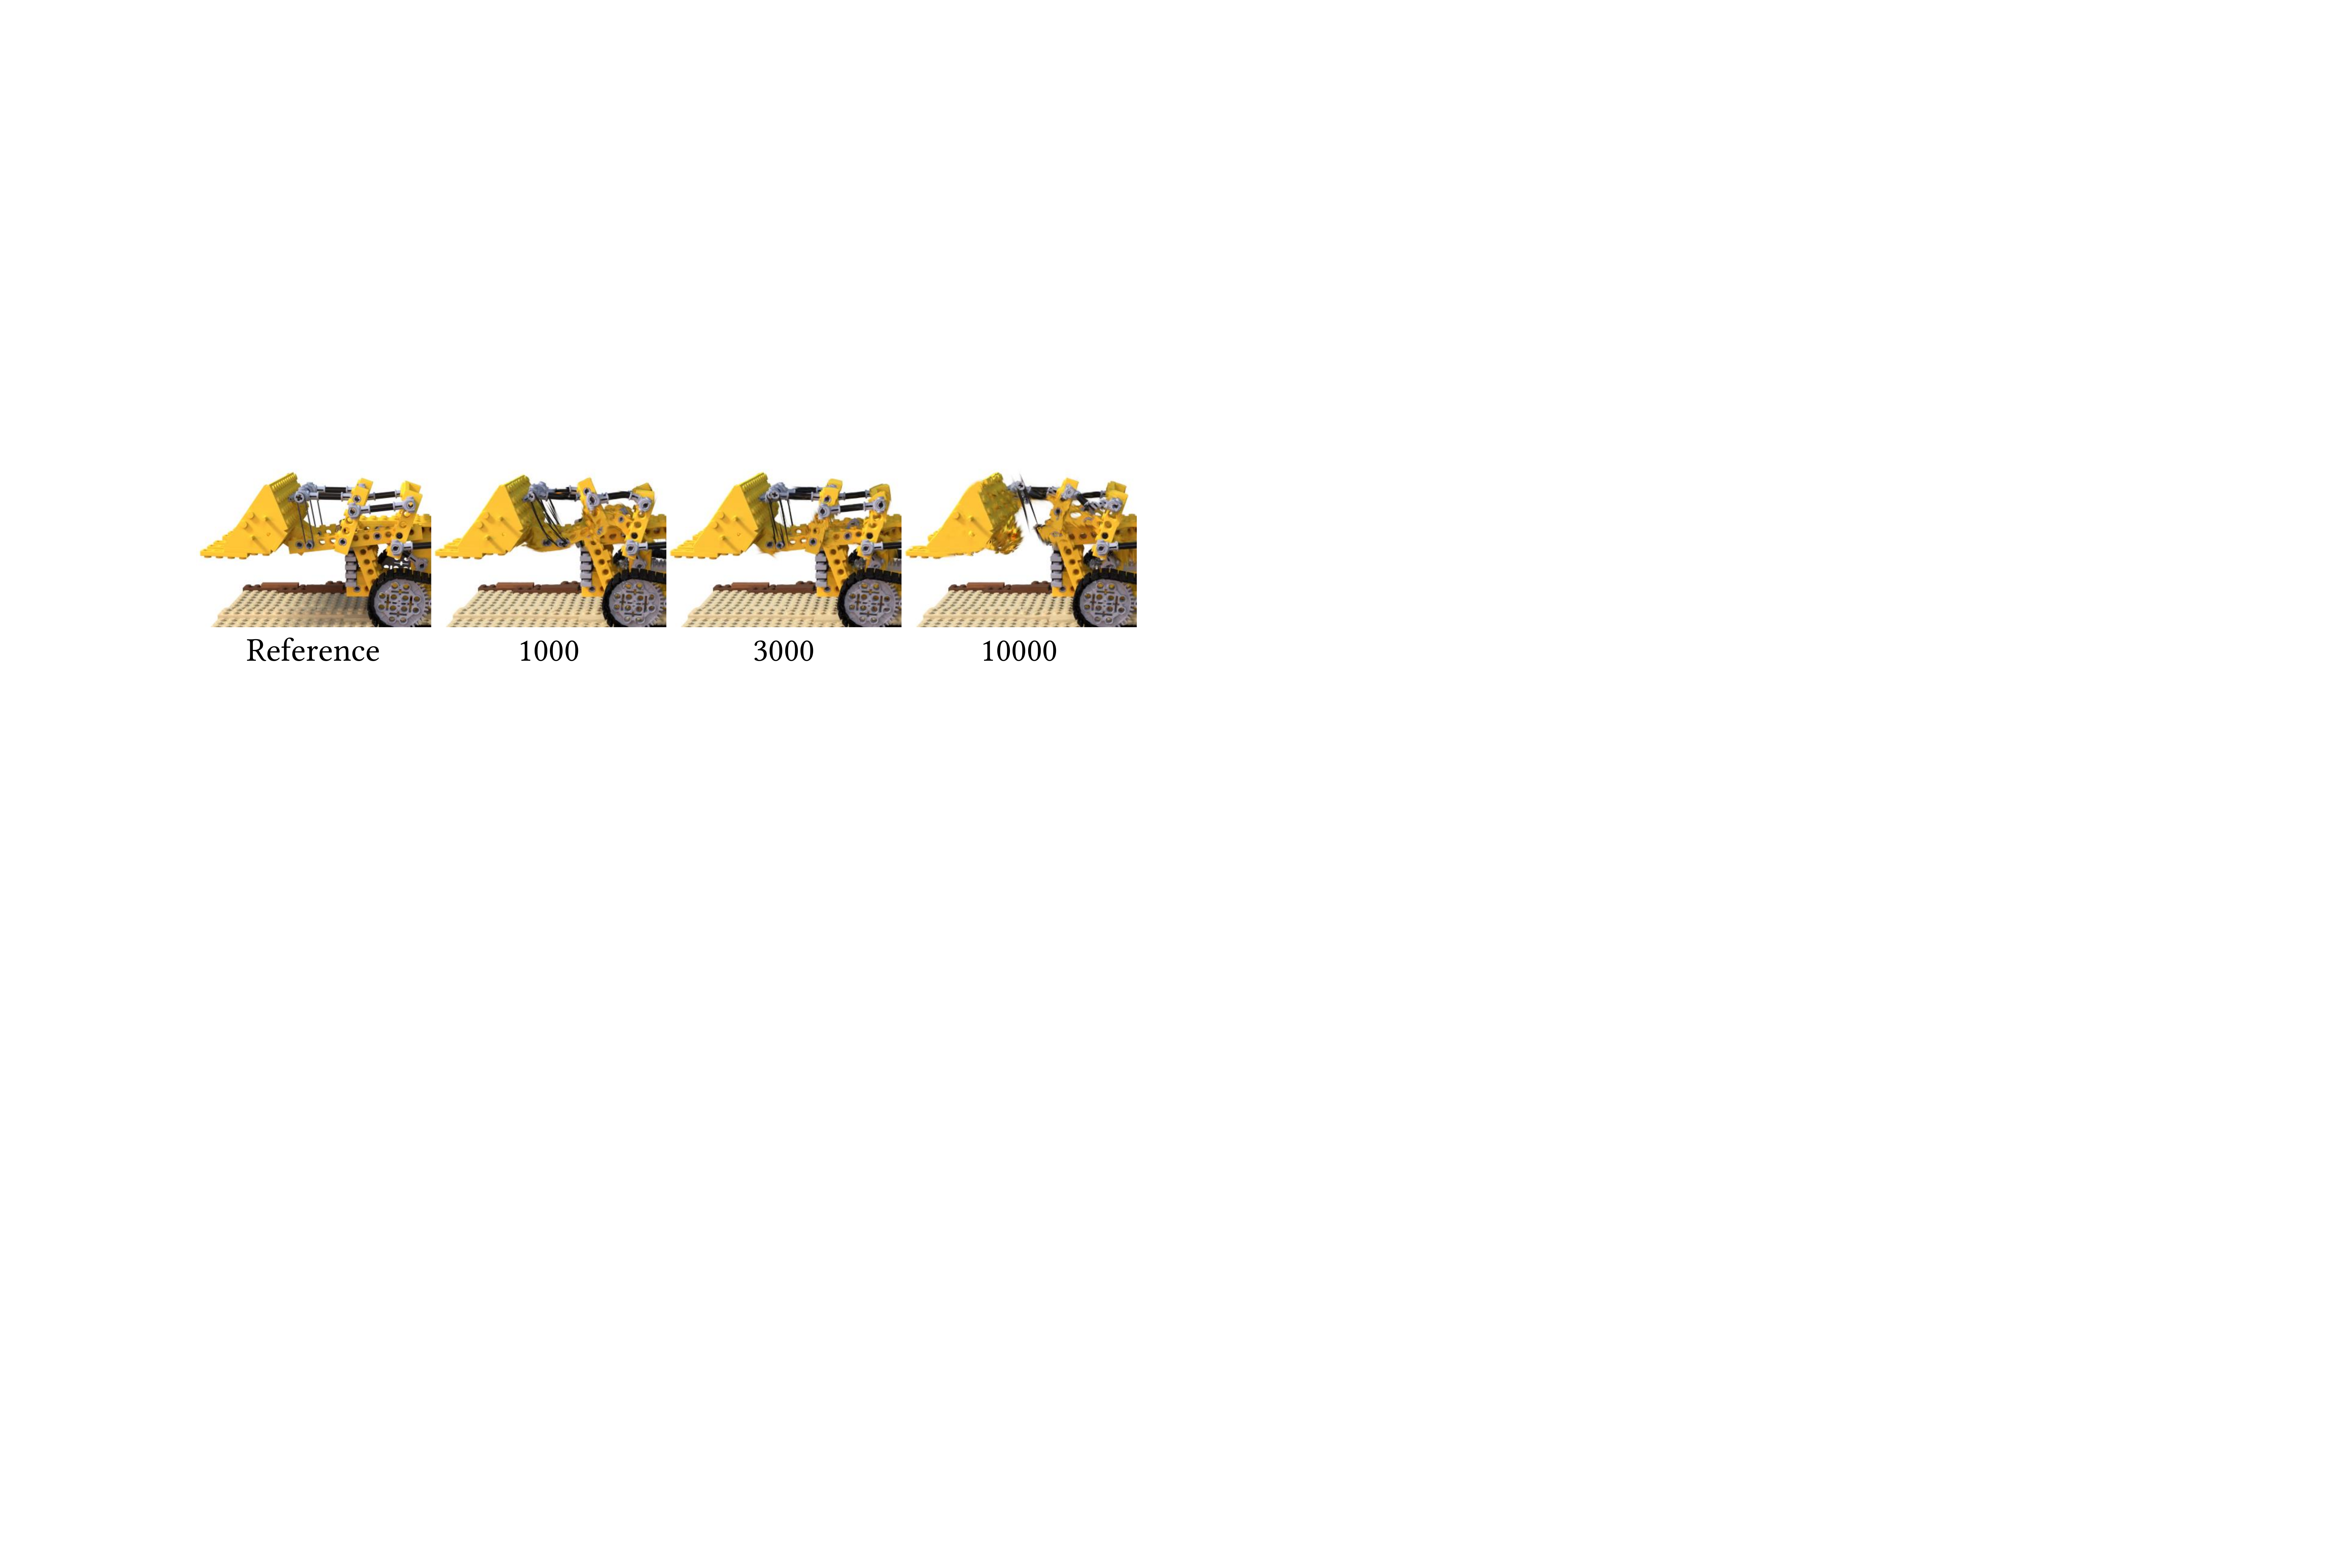}
    \caption{\textbf{Non-rigid deformation results of the coarse stage under different numbers of anchor points.}}
    \label{fig:anchor}
\end{figure}

\subsection{Linear Blend Skinning}

We employ an anchor-based hierarchical structure to model long-range object motions. To be more specific, we derive the deformation field of Gaussians using linear blend skinning (LBS) by locally interpolating the transformations of their neighboring anchor points, expressed as
\begin{align}
\overline\mu_i&=\sum_{j\in\mathcal{N}_i}w_{ij}(R_j^a(\mu_i-a_j)+\overline a_j)\\
    \overline q_i&=(\sum_{j\in\mathcal{N}_i}w_{ij}r_j^a)\otimes q_i
\end{align}
Here, $a_j$ is the initial position of anchor point $j$, $\overline a_j$ denotes the current position, and $\otimes$ is the production of quaternions. For each Gaussian $i$, we use KNN search to obtain its K nearest anchor points, denoted by $\mathcal{N}_i$. We compute the interpolation weight $w_{ij}$ between a Gaussian $G_i$ and an anchor point $A_j$ with RBF. Consequently, we can compute the derivatives with respect to the positions and quaternions of anchor points.

\subsection{Rigidity Mask}

We regularize the overall structural stability with adaptive rigidity constraints. All the regularization terms are defined using the Radial Basis Function(RBF), where the hyper-parameter $\gamma$ for RBF is set to be $5$. We periodically reset the weight mask by taking the maximum value between the weight and a hyper-parameter $\eta$
\begin{equation}
    m_{ij}=\sigma^{-1}(\max(\sigma(m_{ij}), \eta))
\end{equation}
where $\eta$ is set to be $0.99$. We initialize all the rigid masks to be $\sigma^{-1}(0.99)$ and reset them every $3000$ iterations.

\subsection{Loss Function}

In our experiments, we set $\lambda_1 = 3.2$, $\lambda_\text{SSIM}=0.8$, $\lambda_\text{ARAP}=600$, $\lambda_\text{Rotation}=600$, $\lambda_\text{Distance}=30$ and $\lambda_\text{Mask}=0.005$ in the coarse stage and adopt $\lambda_1=0.8$, $\lambda_\text{SSIM}=0.2$, $\lambda_\text{ARAP}=300$, $\lambda_\text{Rotation}=30$, and $\lambda_\text{Distance}=30$ in the fine stage. Additionally, we add $\lambda_\text{scale}=300$ and $\lambda_\text{color}=1.0$ in the fine stage for geometry editing and texture editing, respectively.

\section{Experiment Details}

\subsection{Data Preparation}

For the NeRF Synthetic dataset and Mip-NeRF 360 dataset, we use the original train split to fit the 3D Gaussian model. We select an image from the test split to edit through the 2D imaging tool PhotoShop, including bending the microphone and drum stand, stretching the material ball and hot dog, etc. For the 3DBiCar dataset, we use the same perspective as in NS to render 50 images of the T-pose mesh. We render 8 images of the posed mesh, including one front view, one back view, two side views, and four surround views diagonally above, as shown in Fig.~\ref{fig:posed-mesh}. For the Panoptic Studio dataset, we initialize the scene from the pretrained model from \cite{dynamic-gs}, and then select one video to track the subsequent frames.

\begin{figure}
    \centering
    \includegraphics[width=0.99\linewidth]{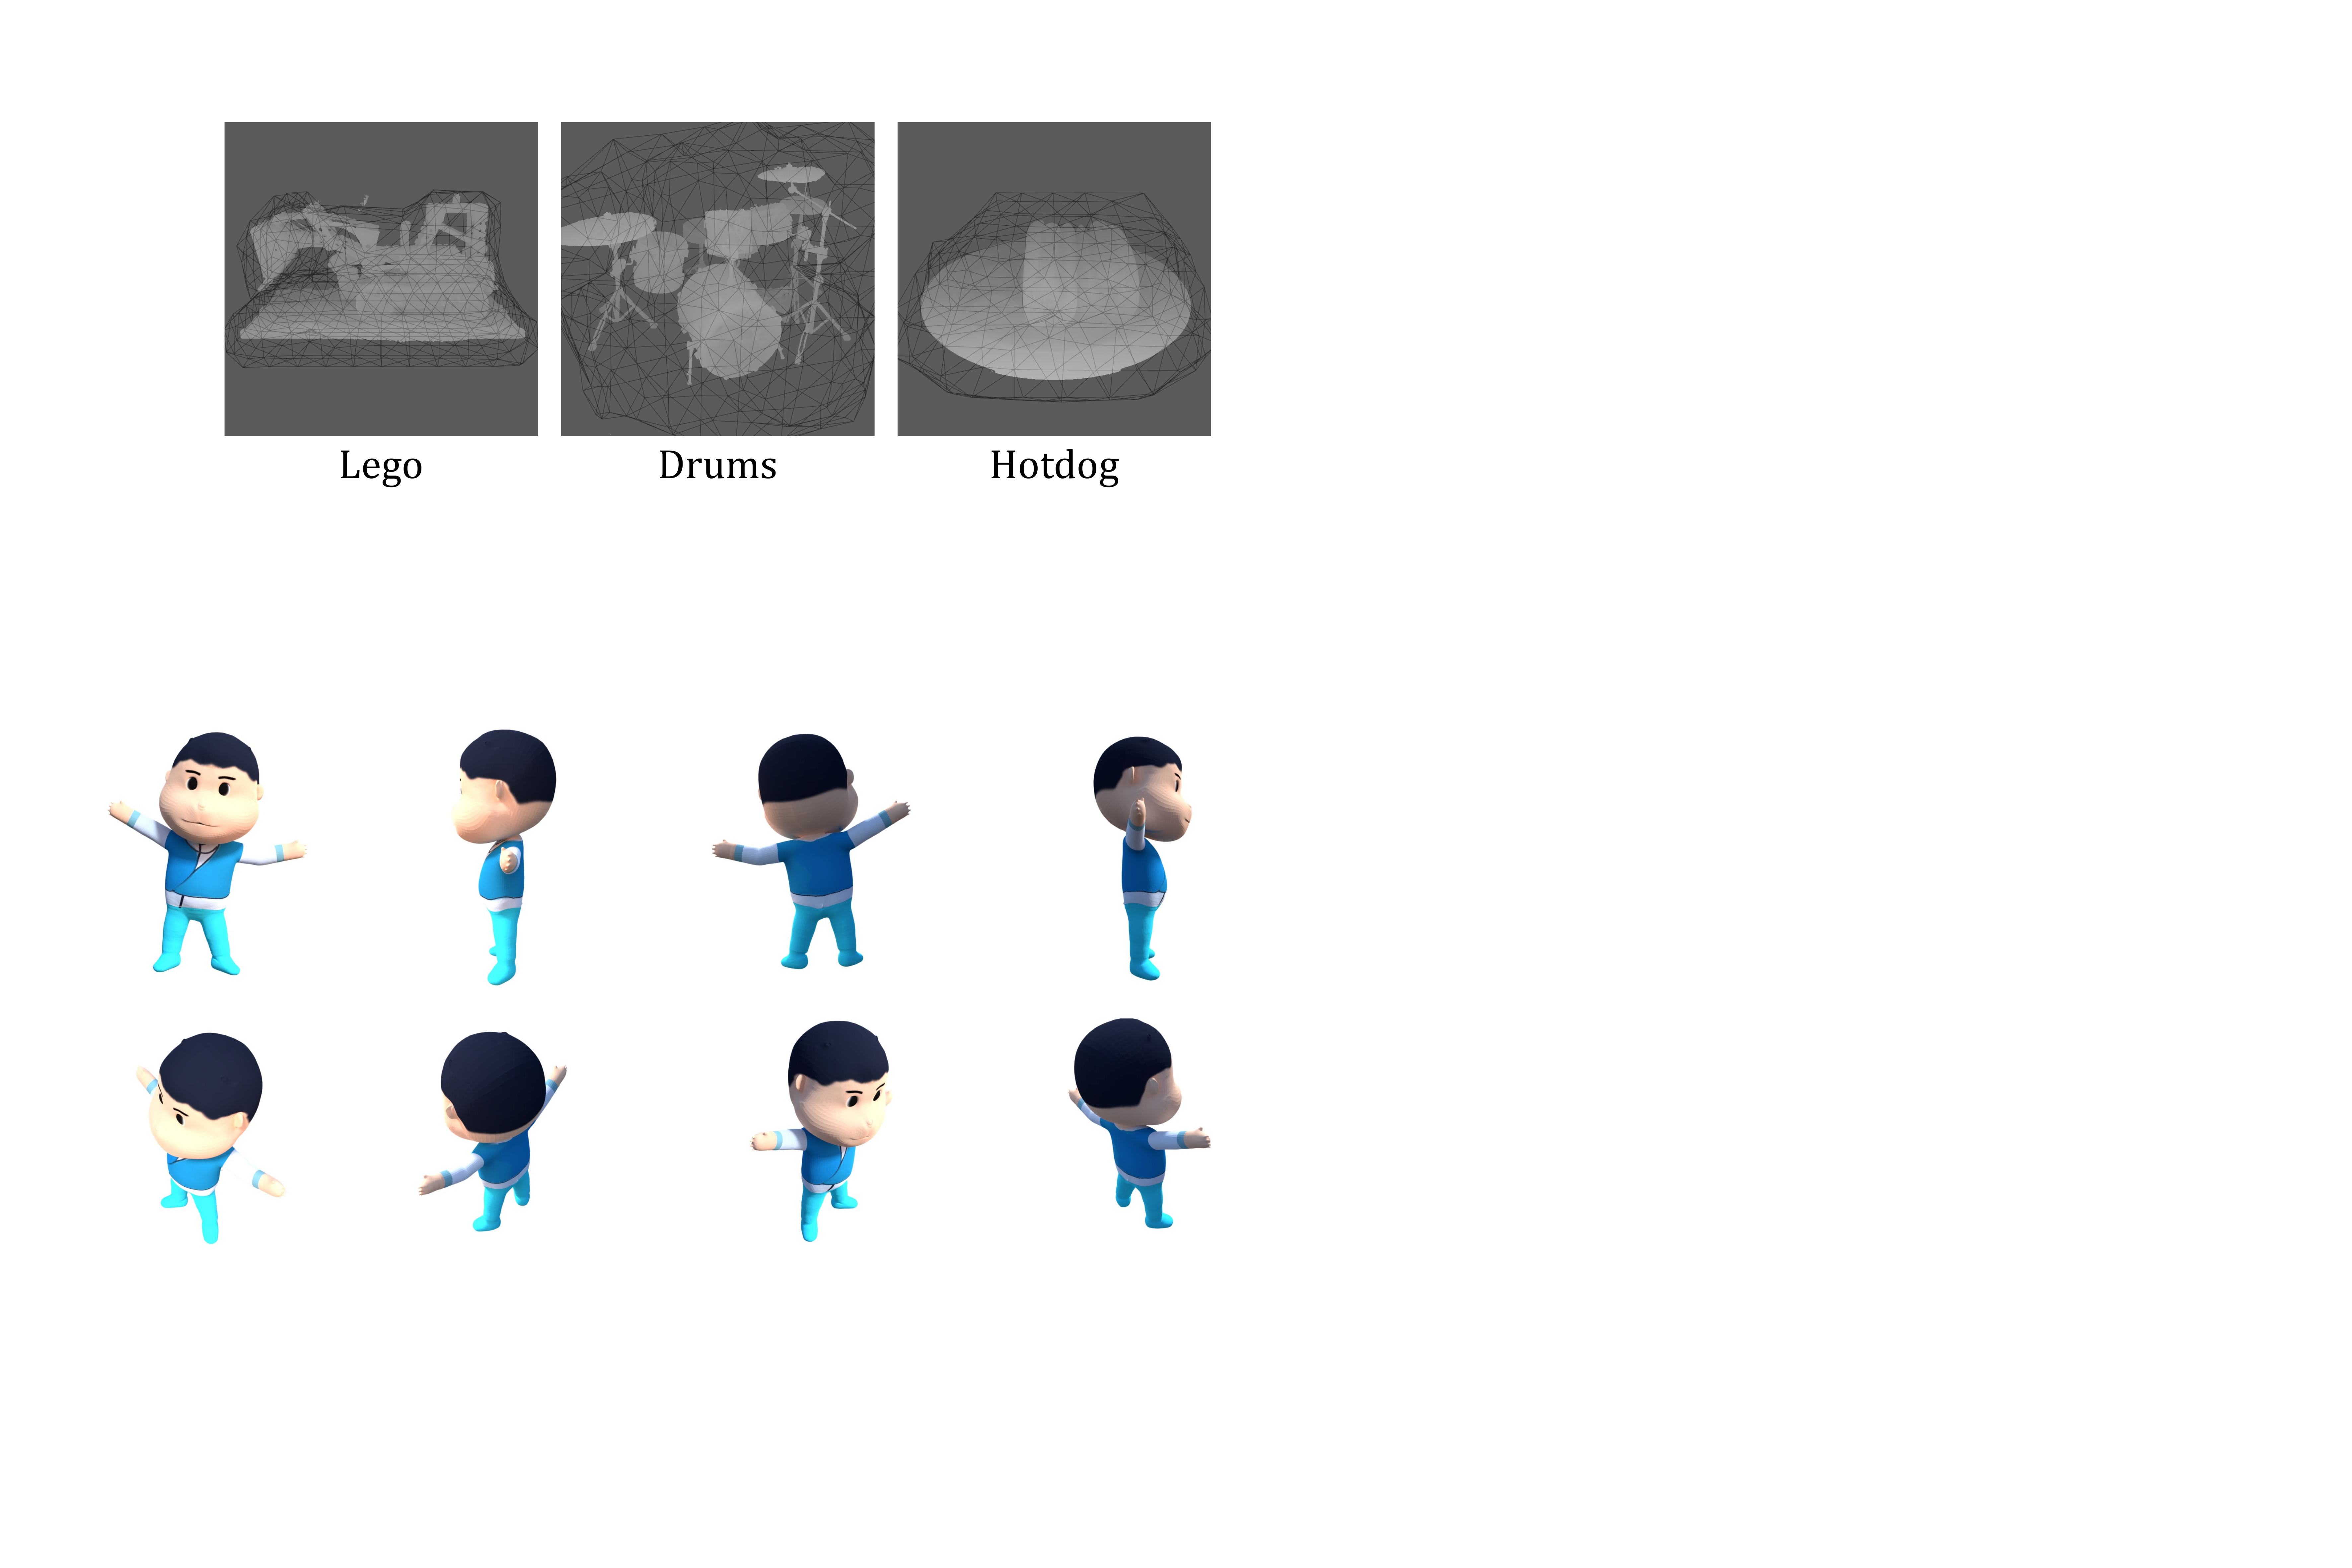}
    \caption{\textbf{Test views of the posed meshes in the 3DBiCar dataset}}
    \label{fig:posed-mesh}
\end{figure}

\subsection{Baseline}

We use vanilla 3DGS, DROT, and Deforming-NeRF as baselines. DROT utilizes mesh as 3D representation and optimizes the mesh vertices. For the NS dataset, we obtain the mesh and the corresponding UV map through NeRF2Mesh\cite{nerf2mesh}. For the 3DBiCar dataset, we directly use the ground truth of the T-pose mesh. Deforming-NeRF fits a NeRF(Plenoxels~\cite{plenoxels}) with multi-view images, extracts the mesh through the Marching Cubes\cite{marching-cube} algorithm, and simplifies it into a cage. Then the user can deform the NeRF by manually adjusting the deformable cage through editing software like Blender. We illustrate the cages extracted from Deforming-NeRF in Fig.~\ref{fig:cage}.

\begin{figure}
    \centering
    \includegraphics[width=0.99\linewidth]{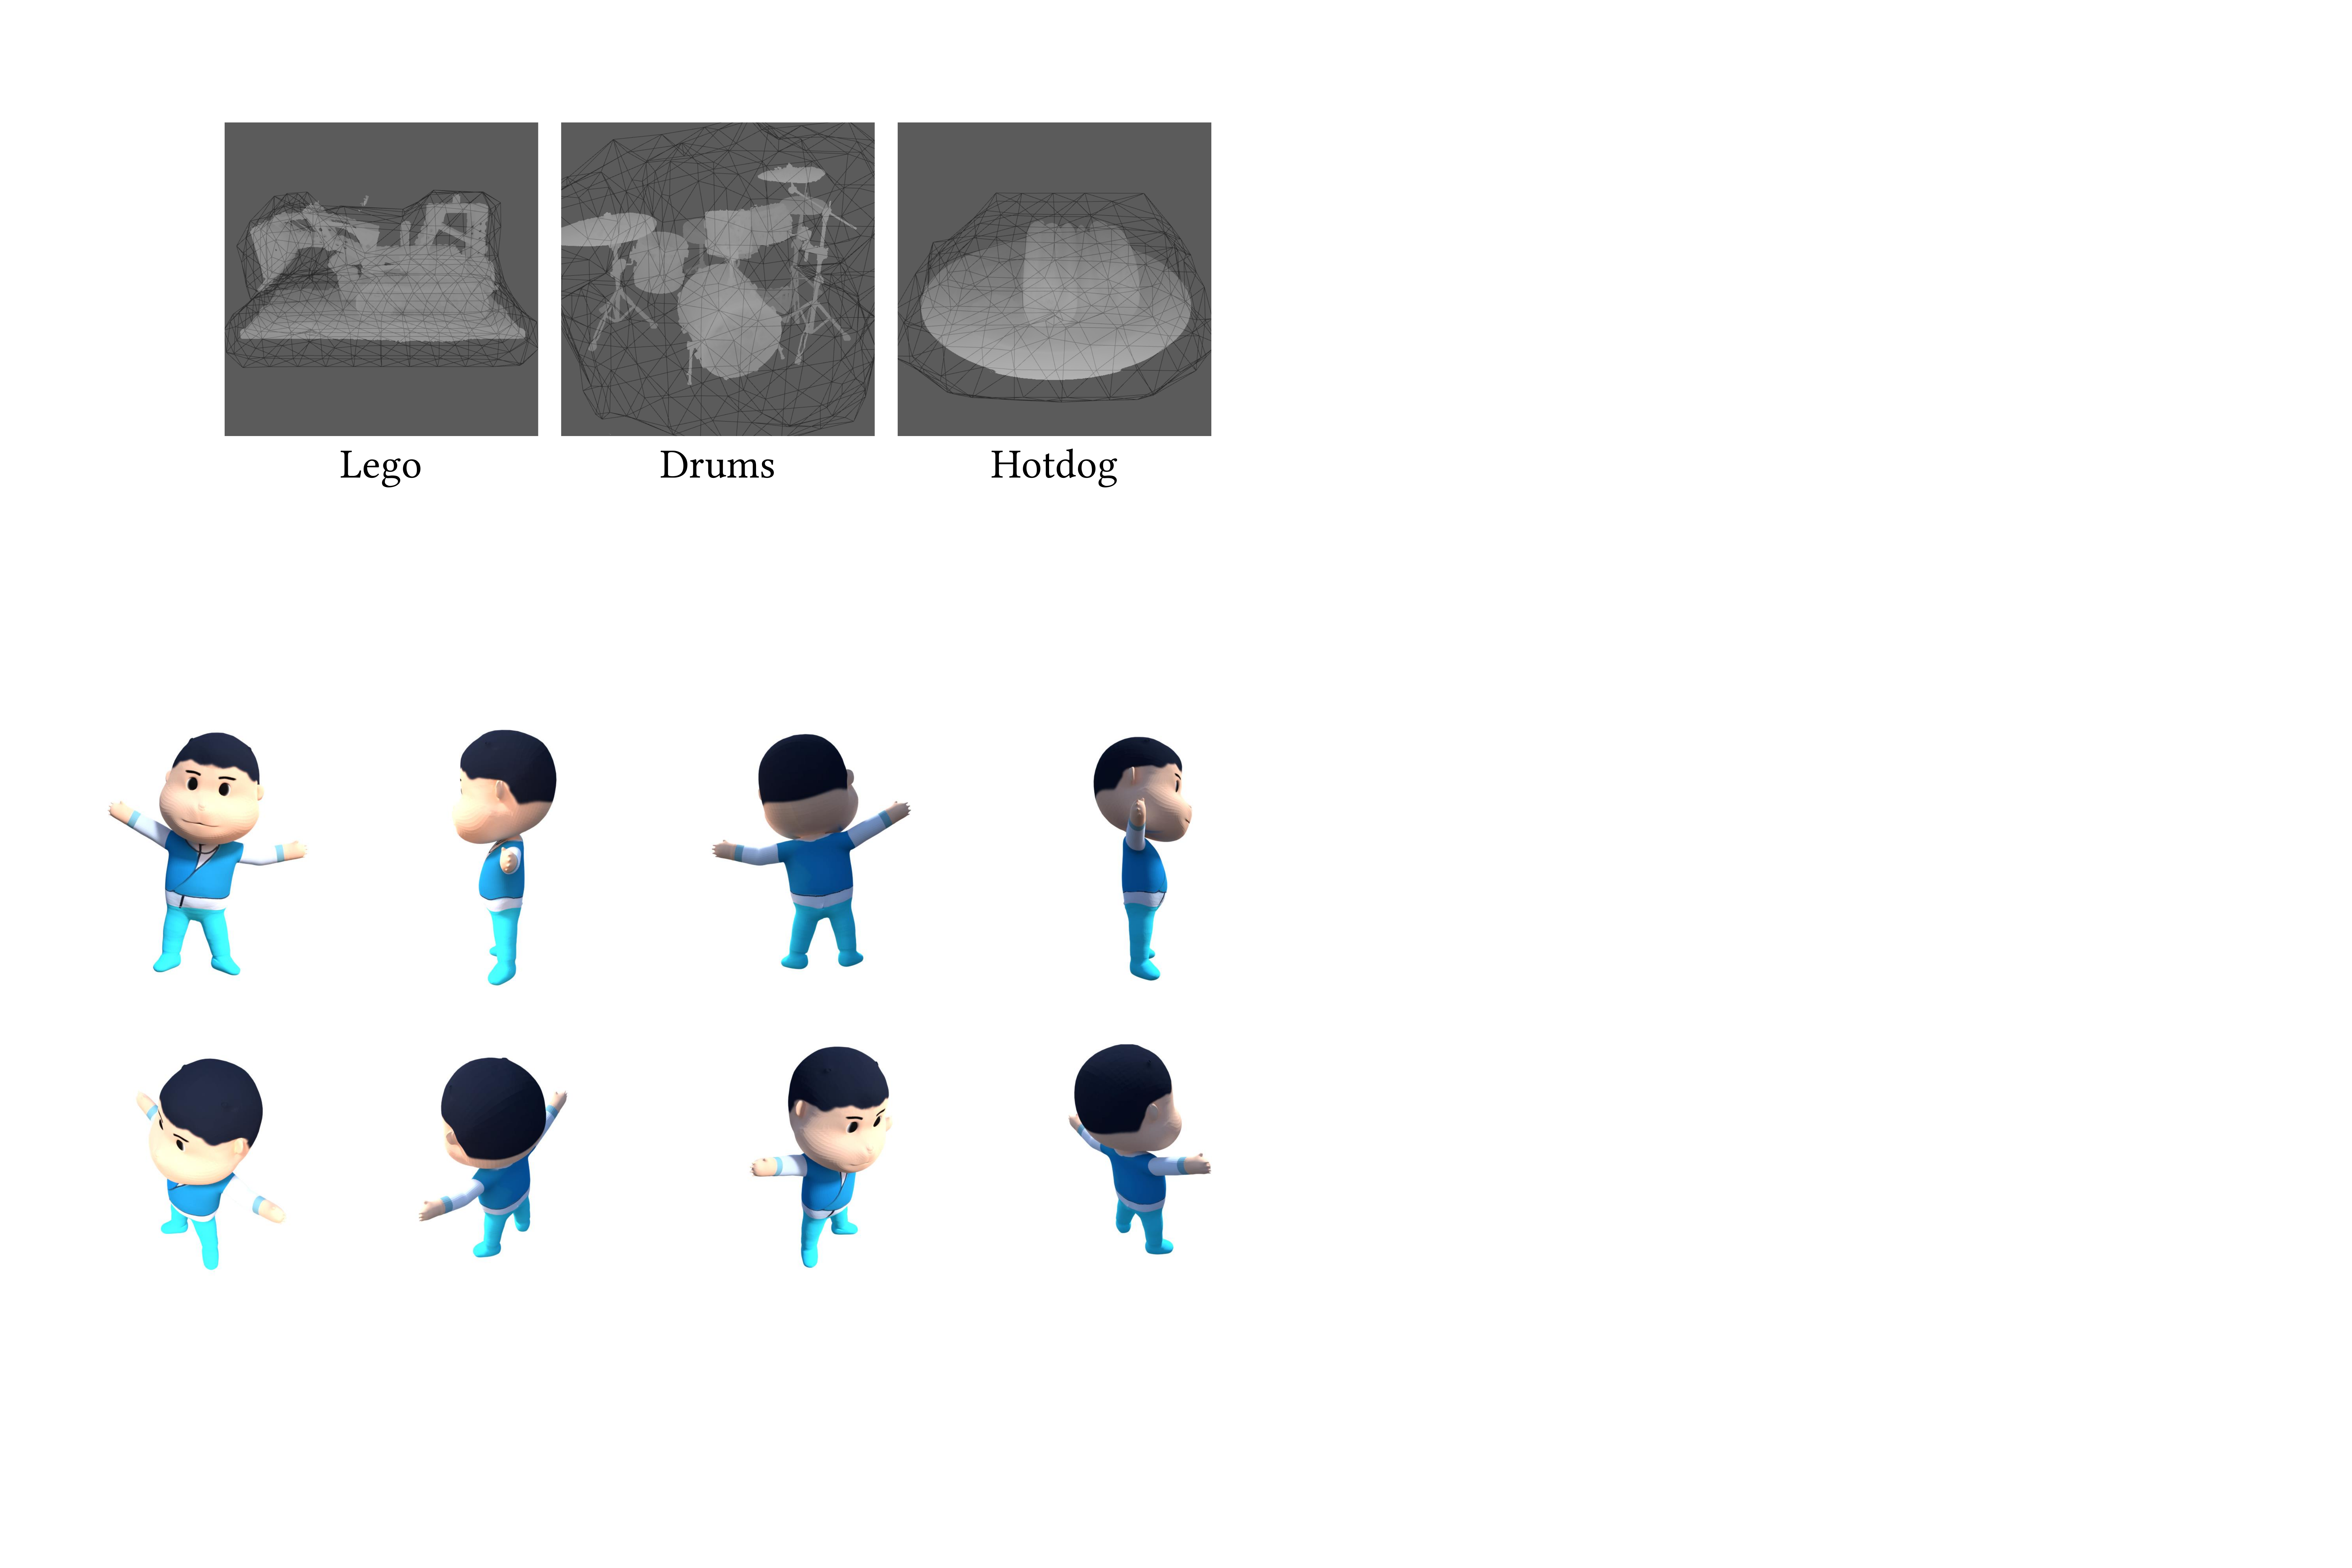}
    \caption{\textbf{Illustration of the extracted cages of Deforming-NeRF on the NS dataset.}}
    \label{fig:cage}
\end{figure}

\section{Application}

We can use image-to-video models, AnimateAnyone~\cite{animateanyone} to generate a video of cartoon characters from a fixed perspective. We then use the video to drive the 3D model frame by frame, thereby generating a dynamic 3D scene. We show results from different frames and different perspectives in Fig.~\ref{fig:application}.

\begin{figure}
    \centering
    \includegraphics[width=0.99\linewidth]{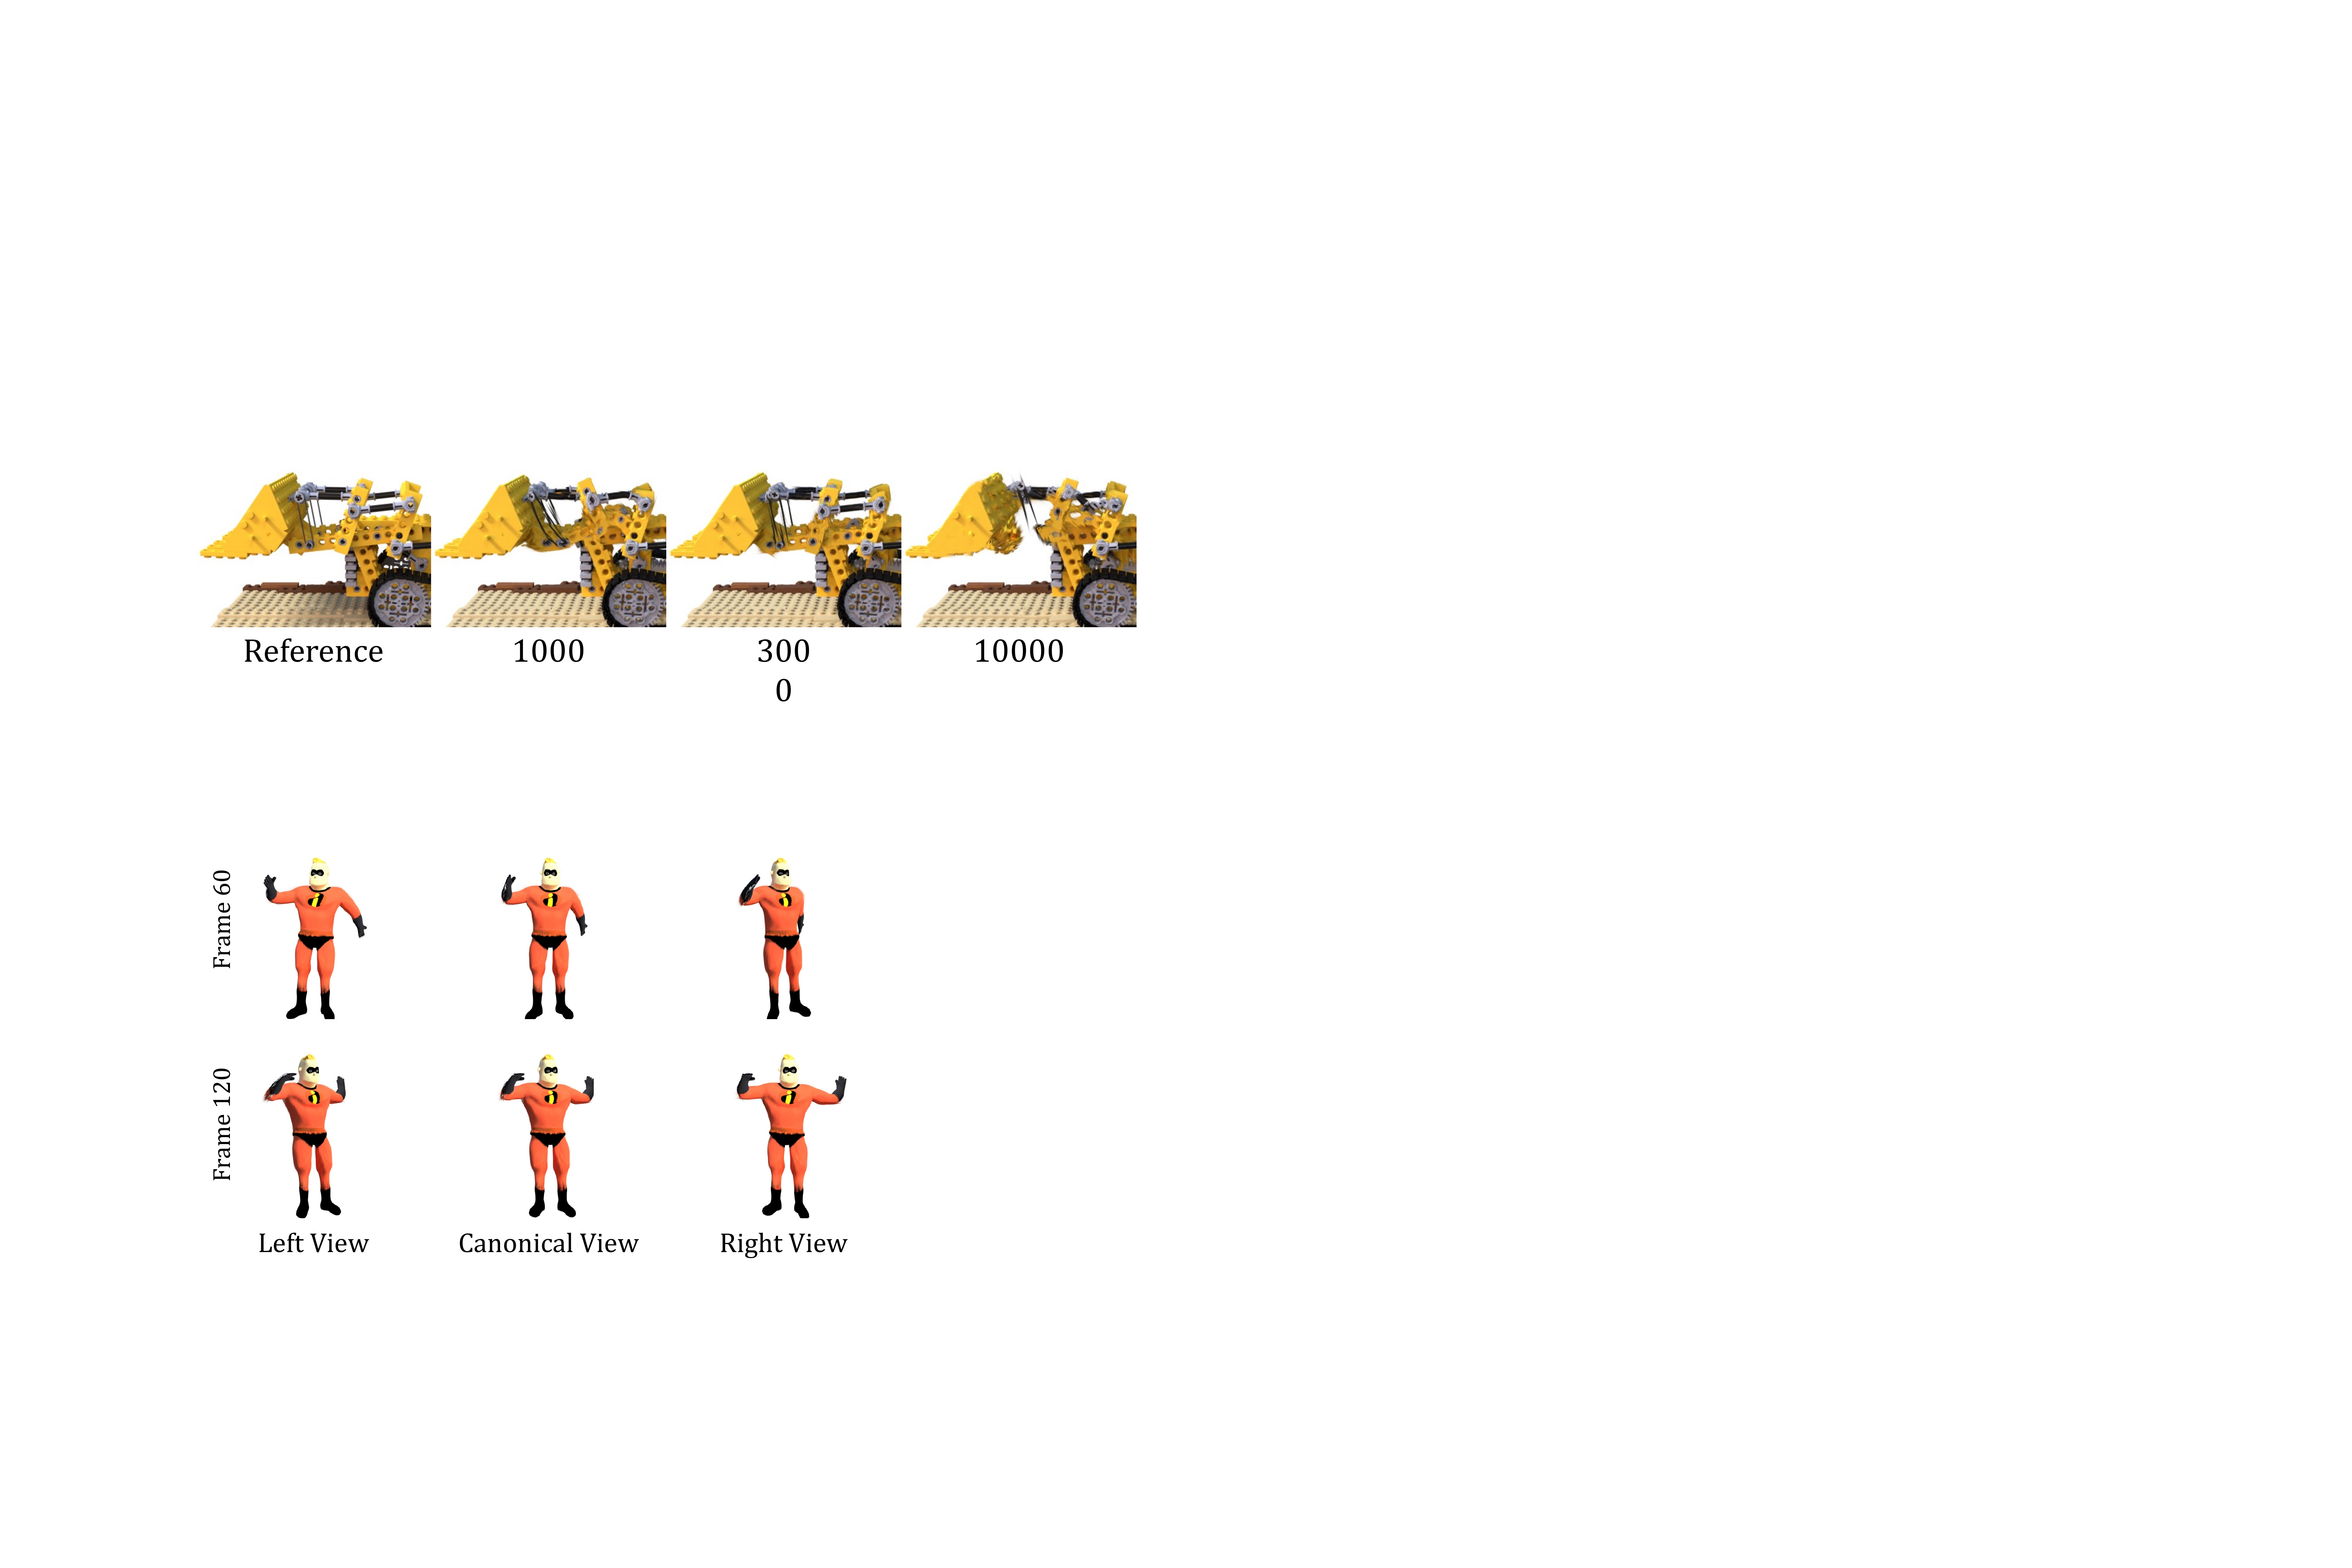}
    \caption{\textbf{The rendered results of the 3D scene from different frames and different views.}}
    \label{fig:application}
\end{figure}
