# Supplementary material for: 3D Gaussian Editing with A Single Image
Source: arXiv:2408.07540 source file (2024-08-14)
Supplement: Supplementary file 2 [file 8_appendix.tex]

\appendix

\begin{figure*}
    \centering
    \includegraphics[width=0.9\linewidth]{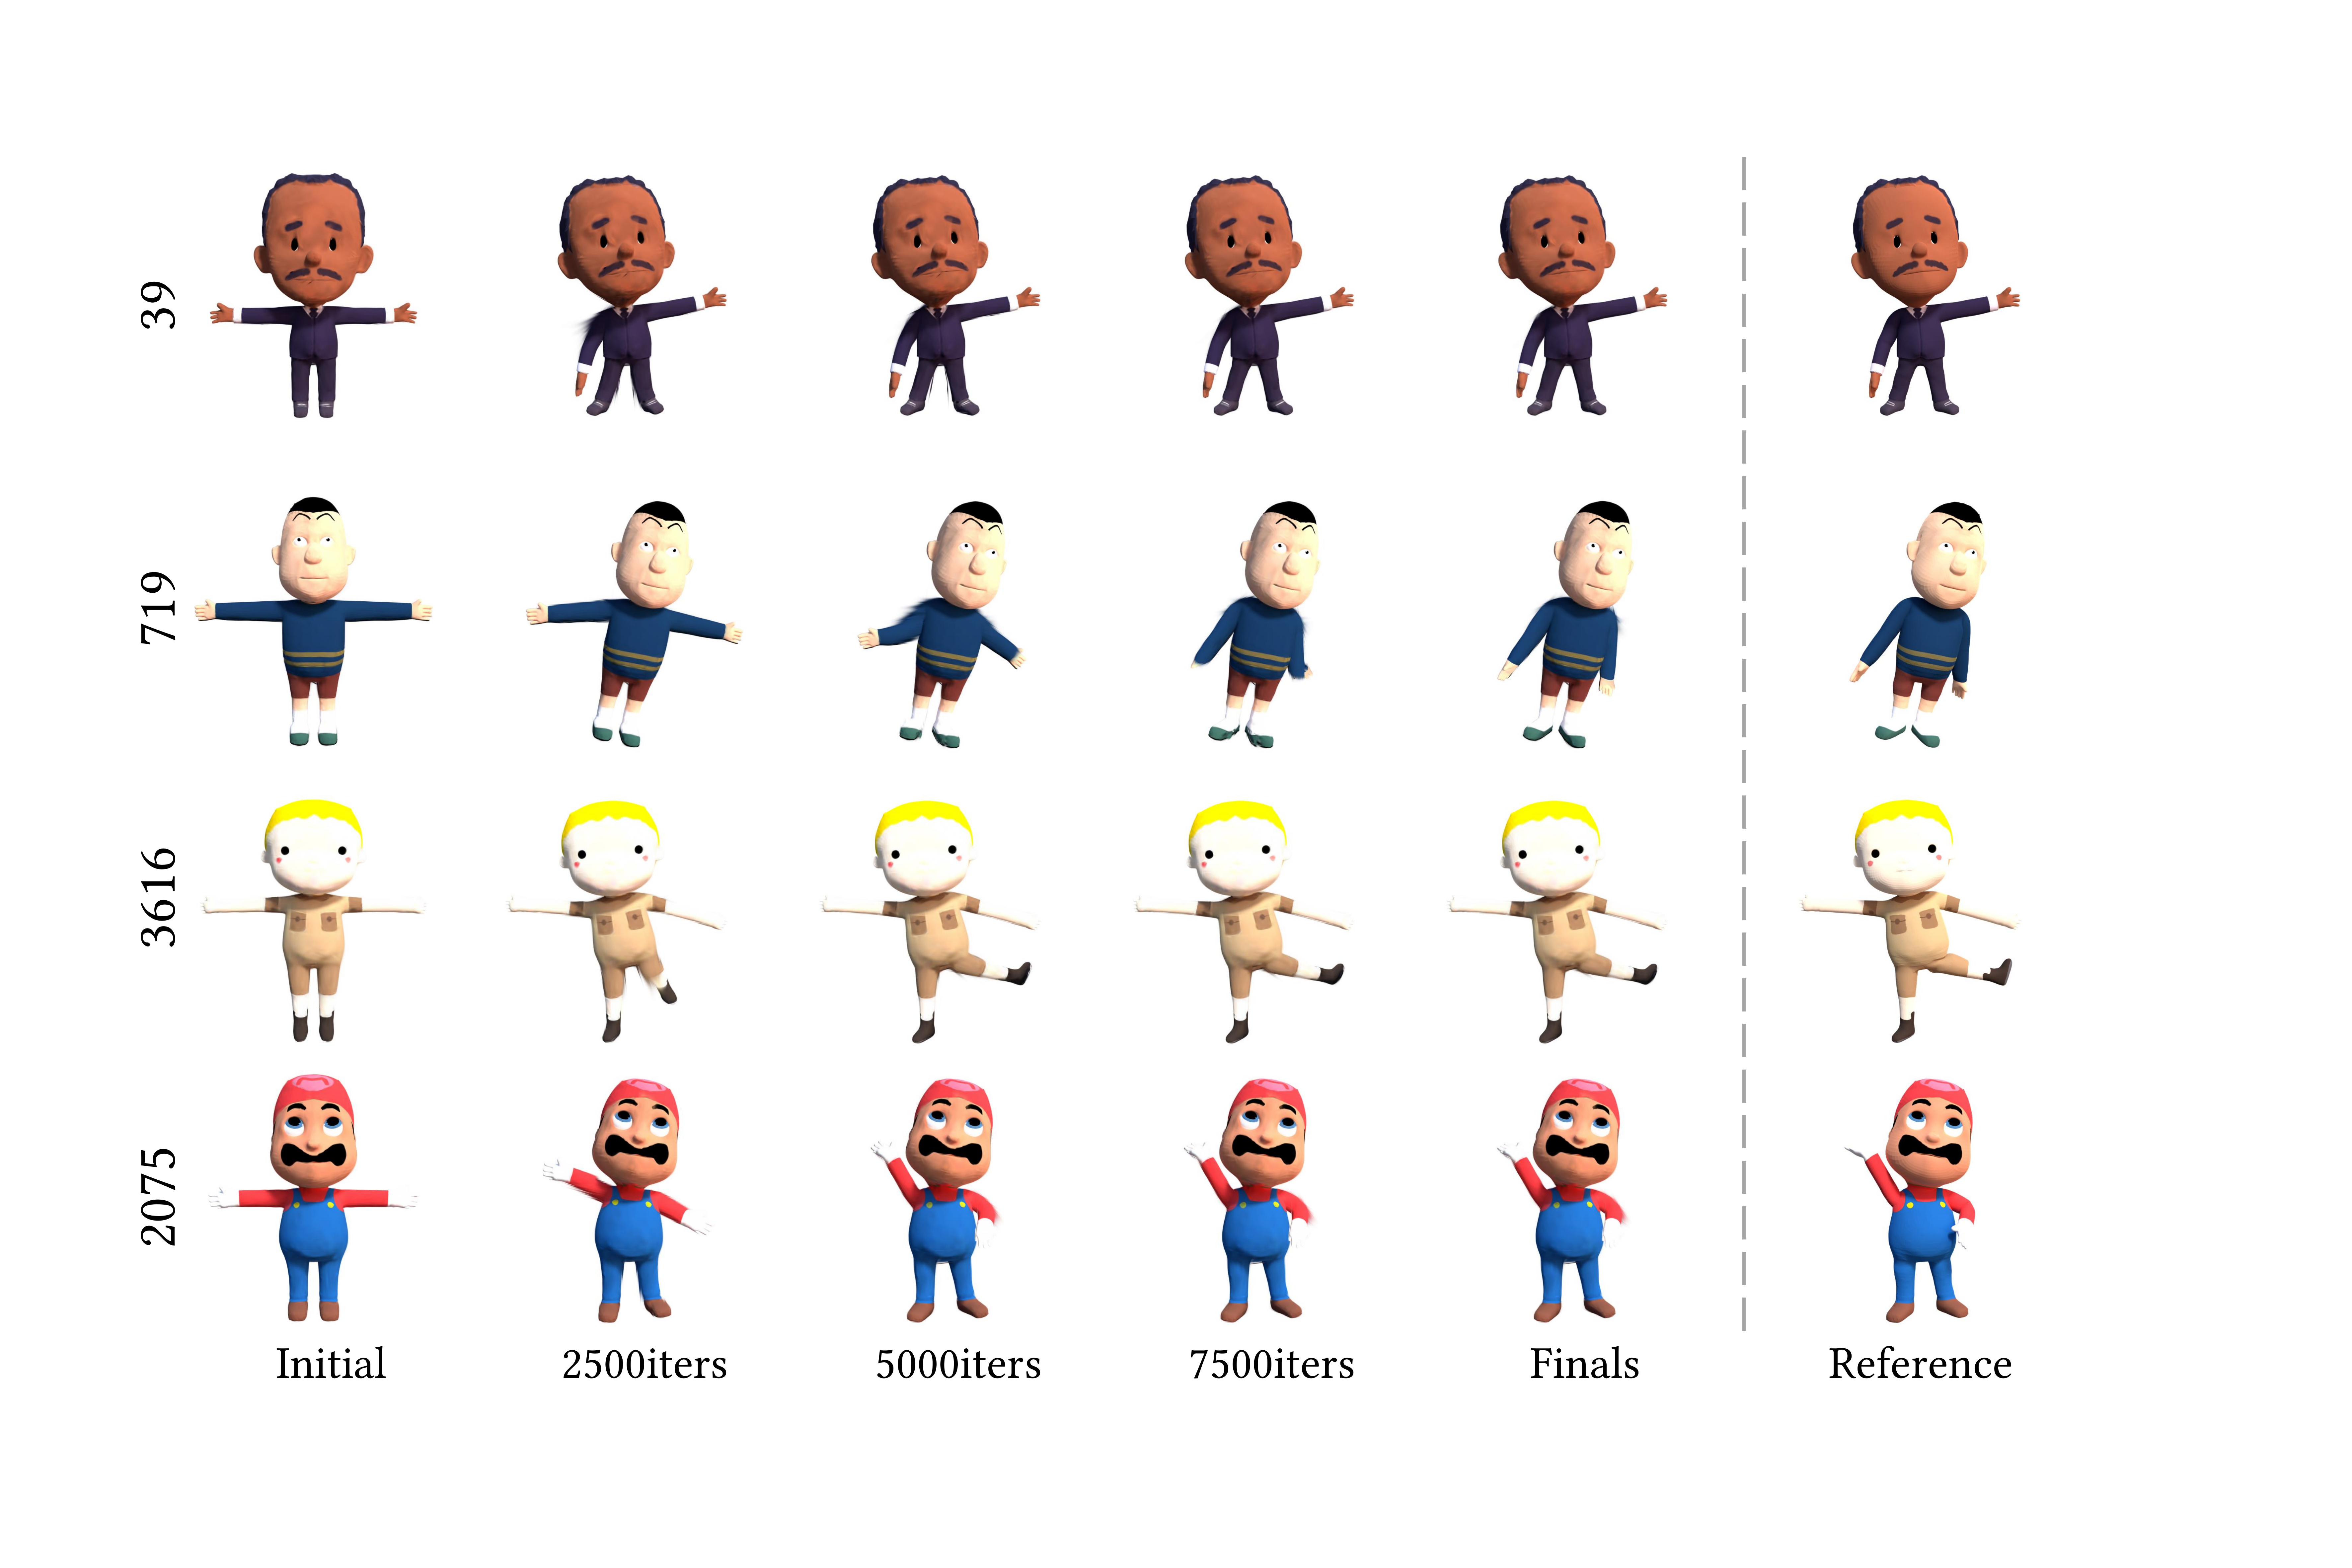}
    \caption{\textbf{Optimization process on 3DBiCar dataset.} We optimize each case for 10,000 iterations(including 6000 iterations in the coarse stage and 4000 iterations in the fine stage) which takes about 2 minutes.}
    \label{fig:appendix-opt-3dbicar}
\end{figure*}

\begin{figure*}
    \centering
    \includegraphics[width=0.9\linewidth]{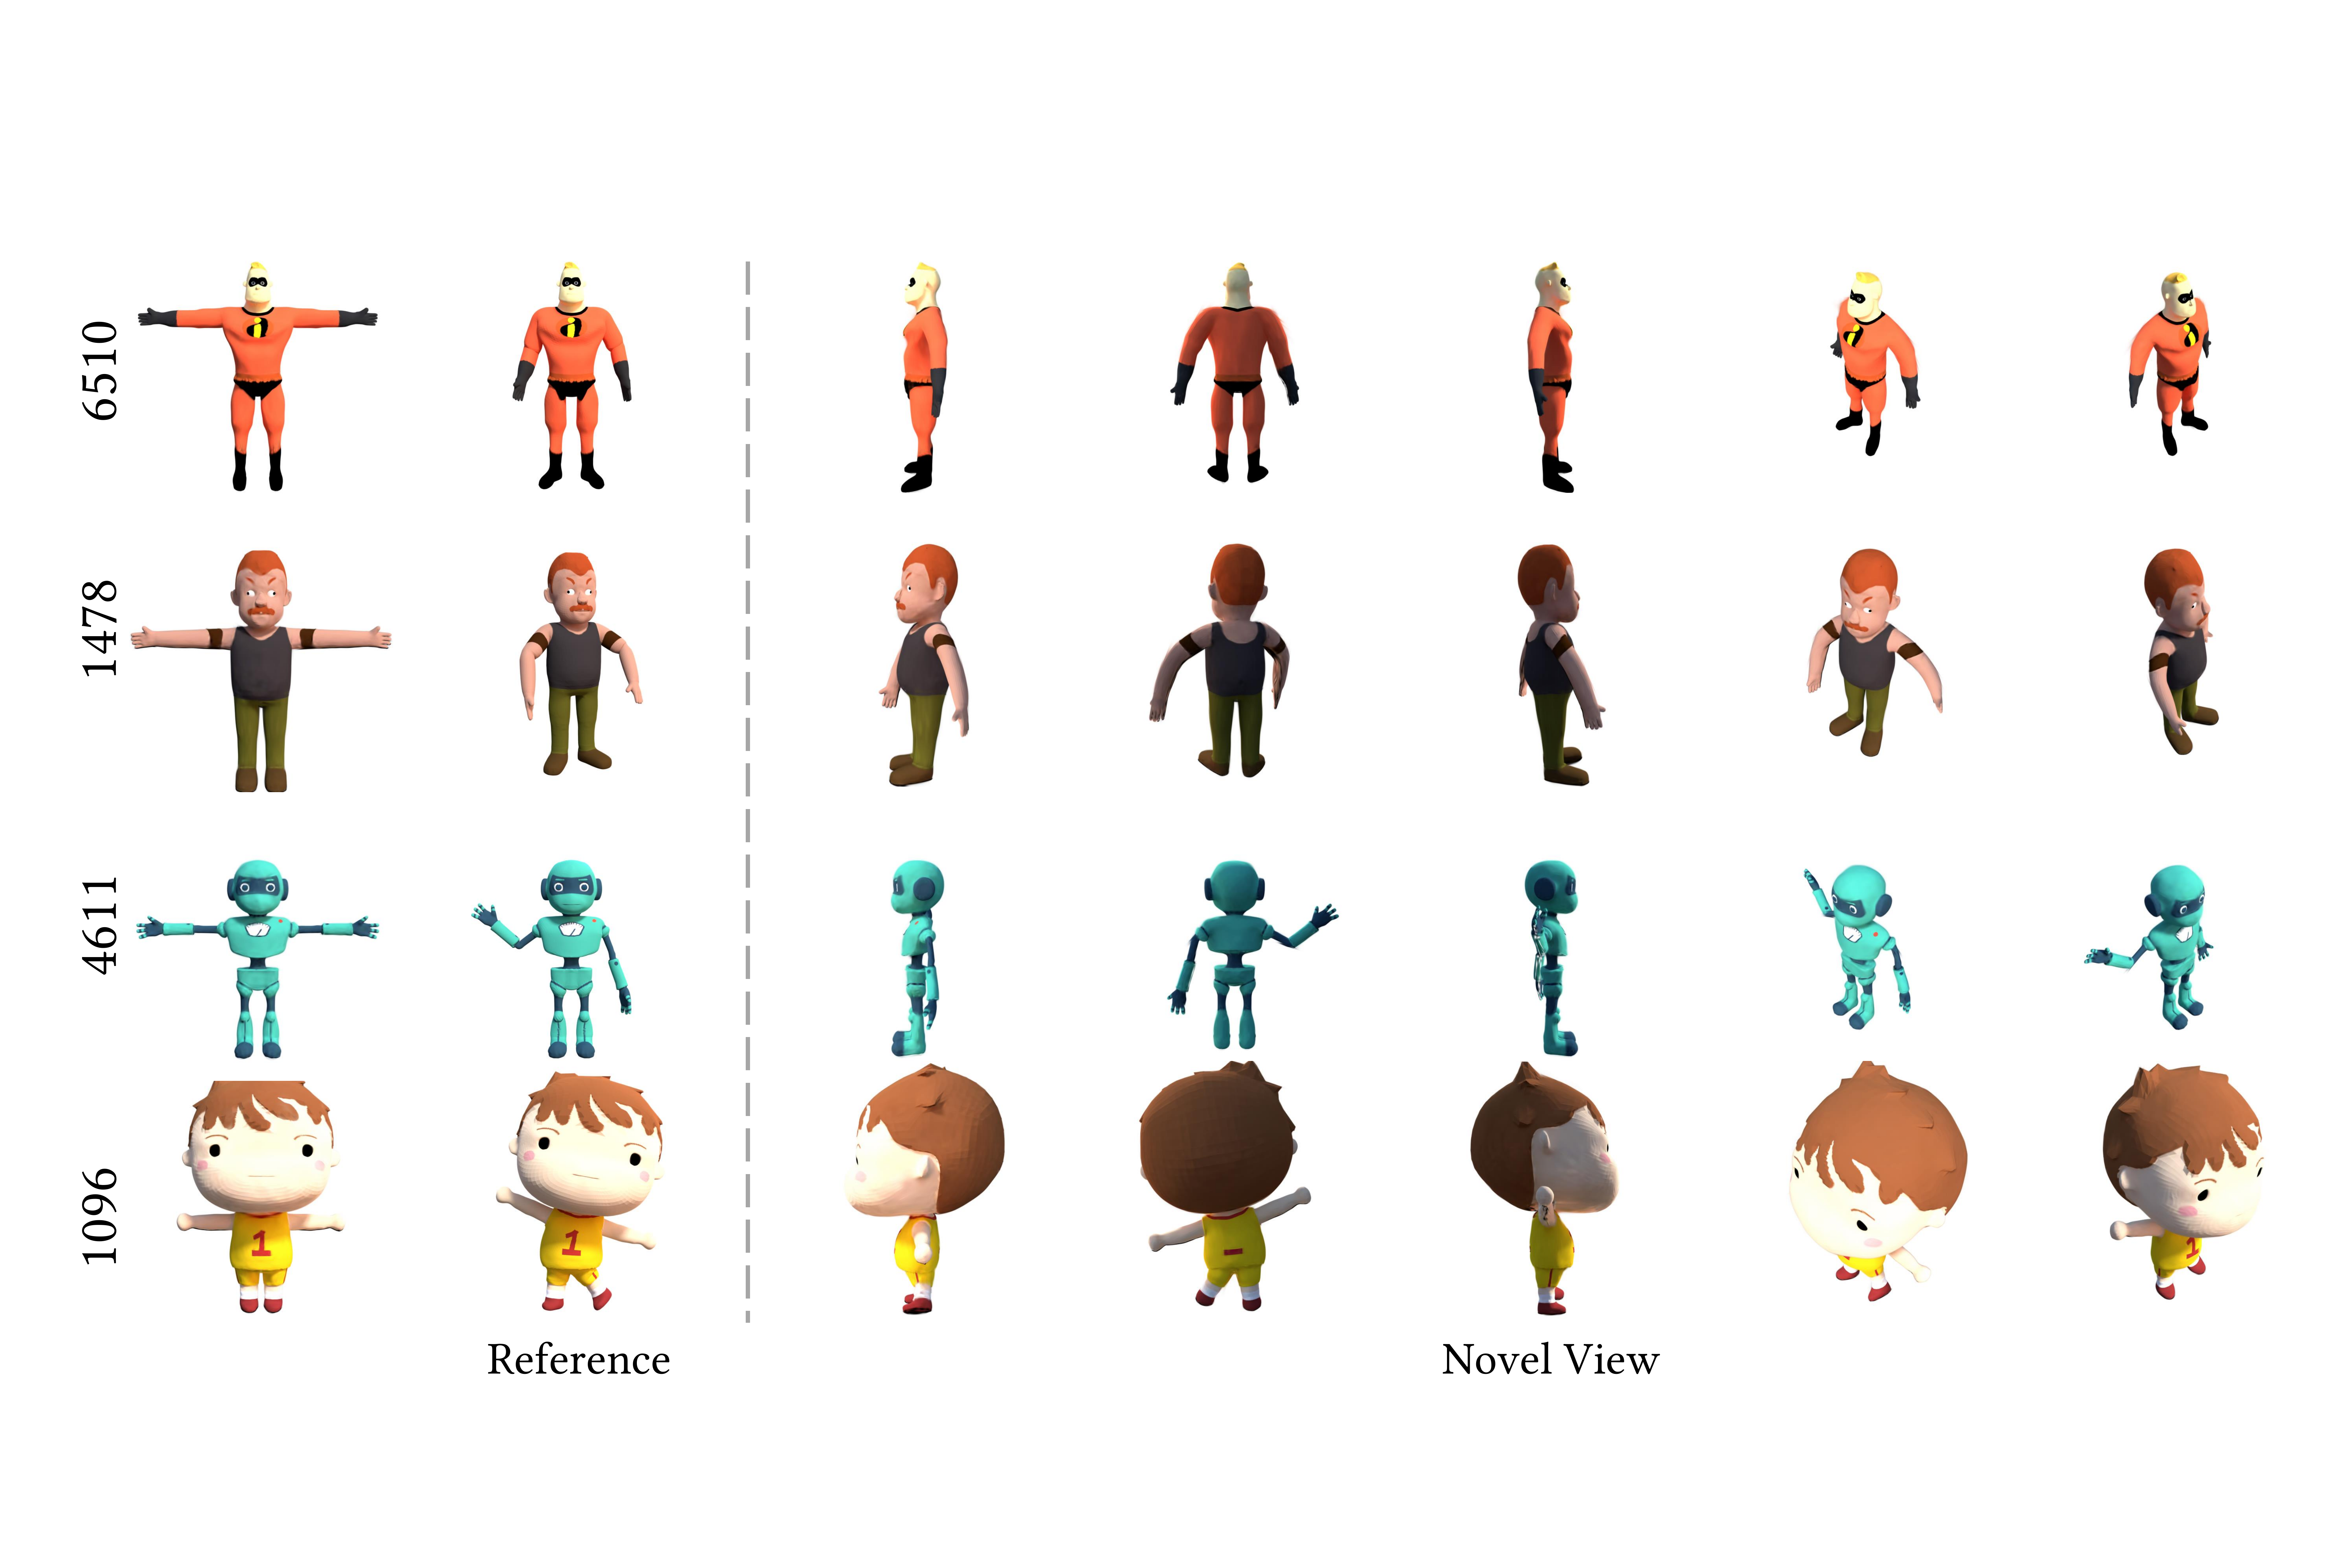}
    \caption{\textbf{Novel view results on 3DBiCar dataset.} 
    % Our method can achieve 3D consistency while maintaining structural stability thanks to the anchor-based structure and two-stage optimization strategy.
    }
    \label{fig:appendix-nvs-3dbicar}
\end{figure*}

\begin{figure*}
    \centering
    \includegraphics[width=0.95\linewidth]{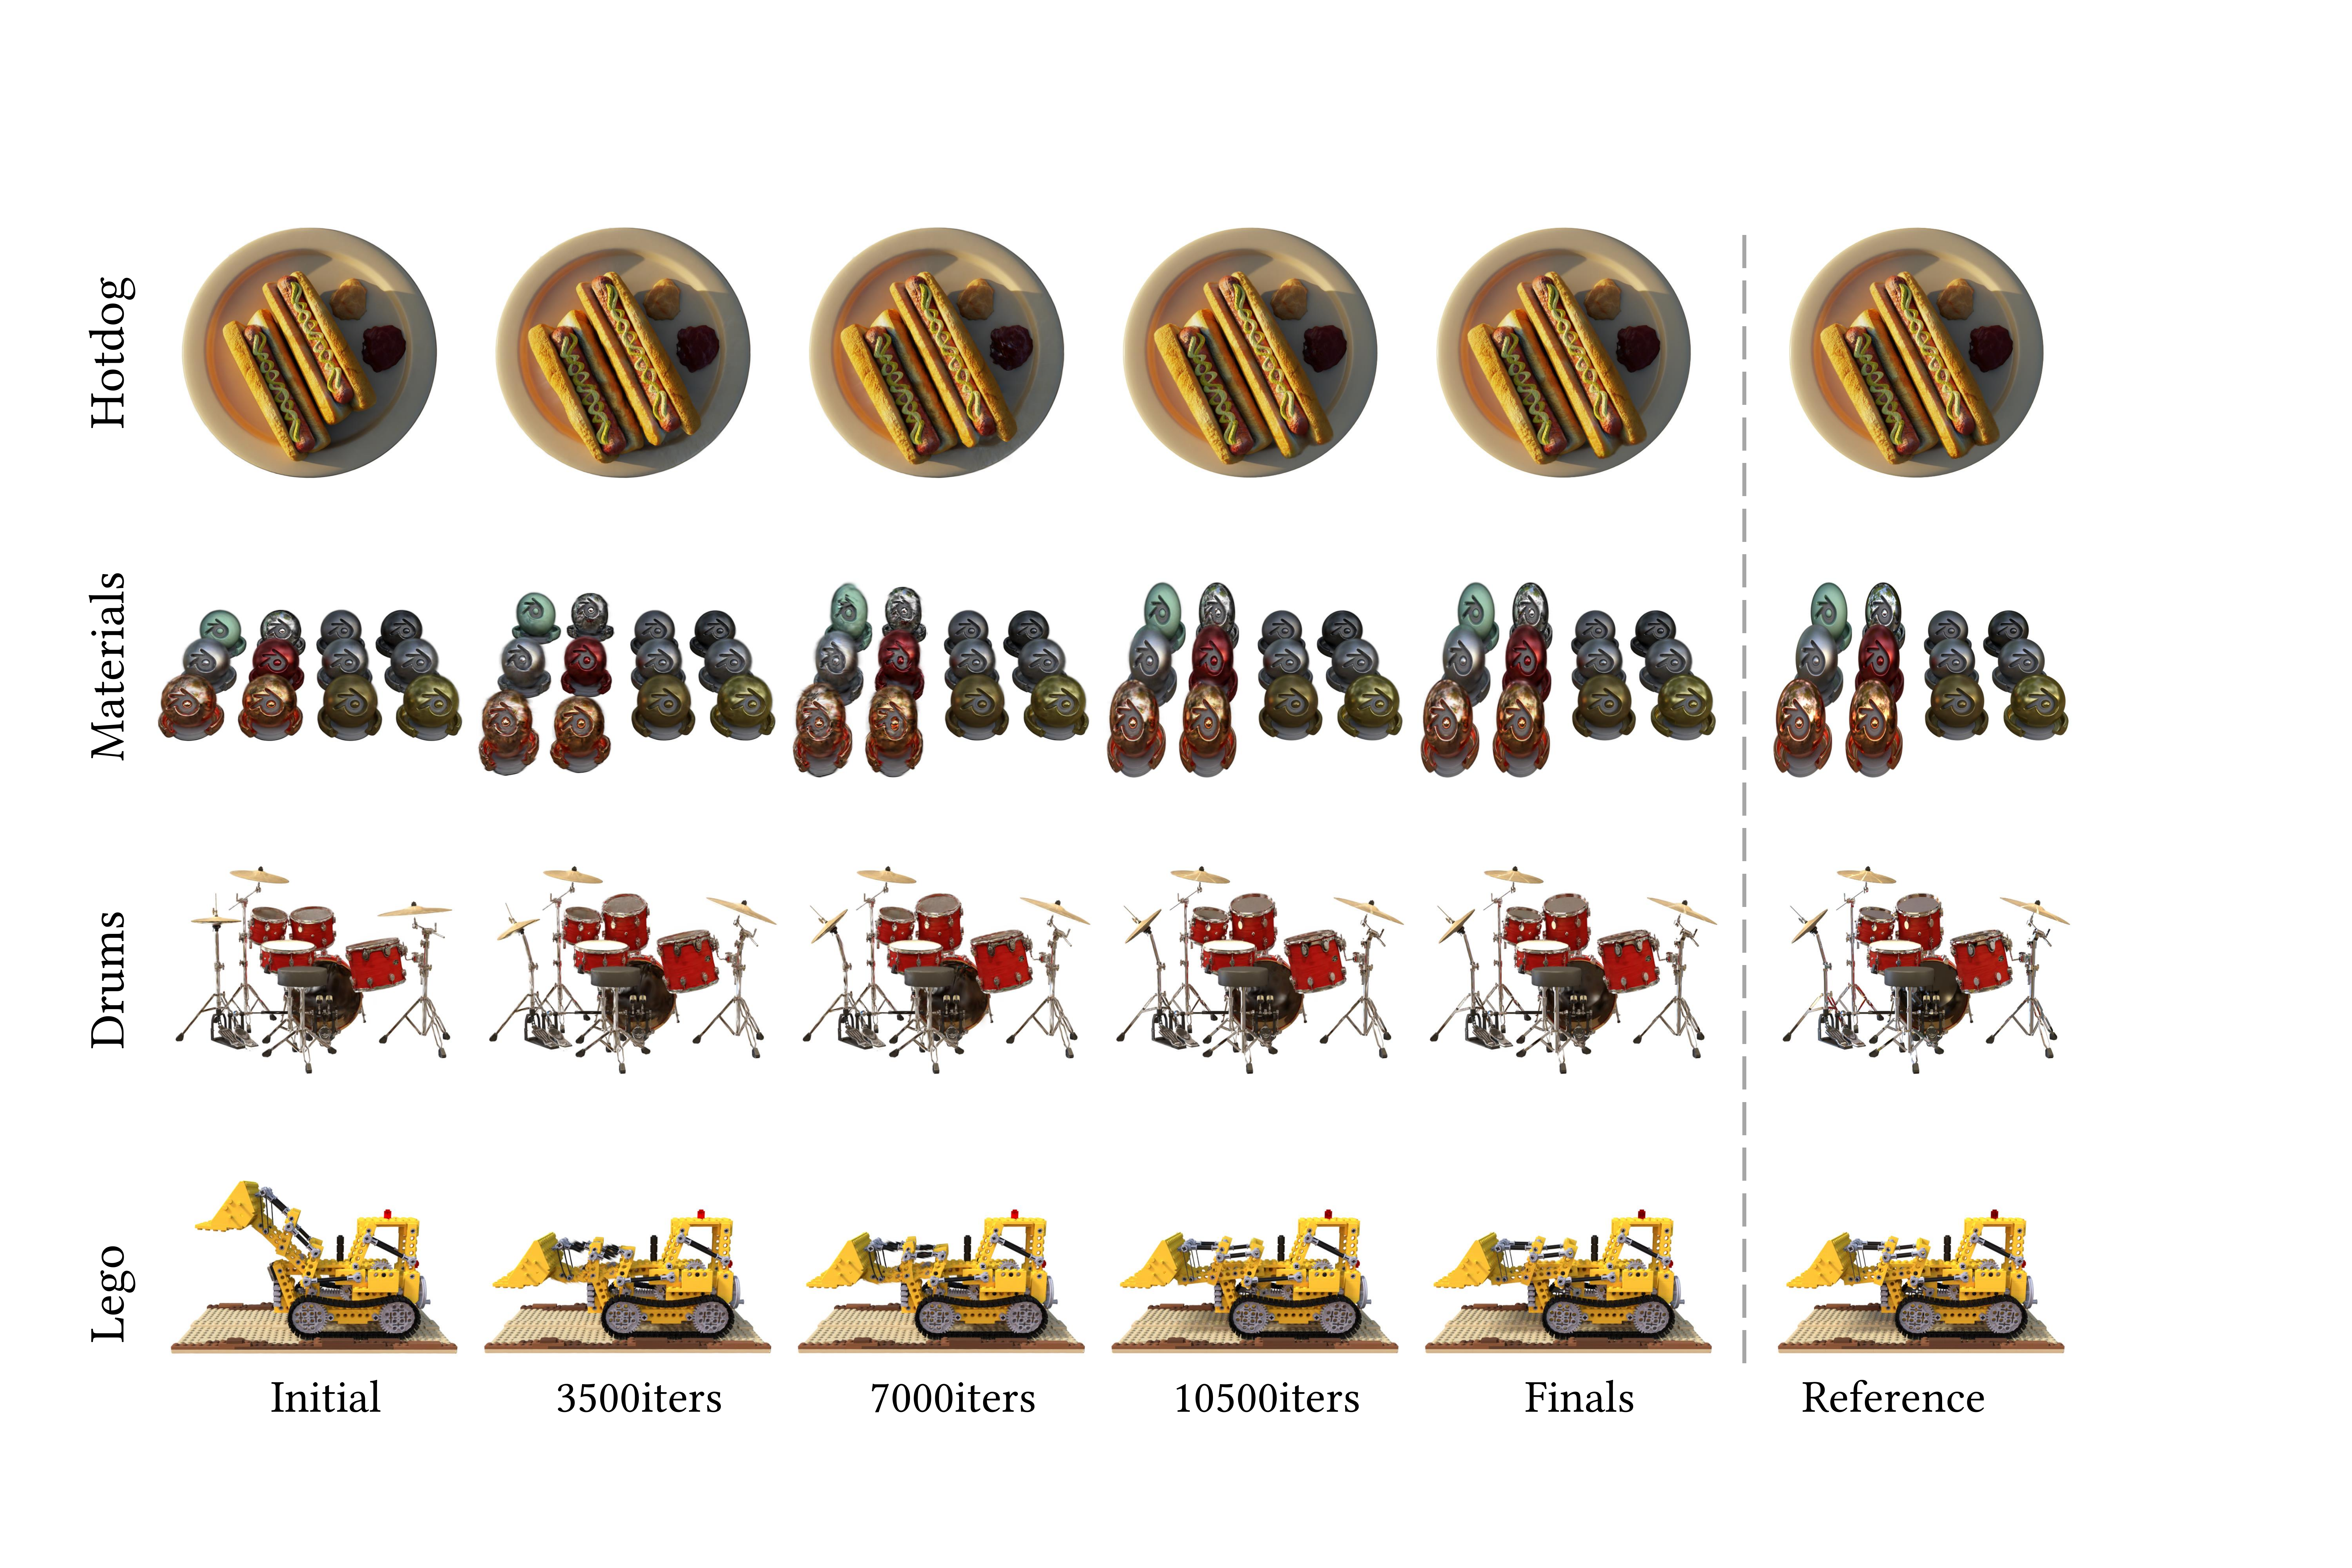}
    \caption{\textbf{Optimization process on NS dataset.} We train each case for 14,000 iterations(including 10000 iterations in the coarse stage and 4000 iterations in the fine stage) which takes about 4 minutes.}
    \label{fig:appendix-opt-nerf}
\end{figure*}

\begin{figure*}
    \centering
    \includegraphics[width=0.95\linewidth]{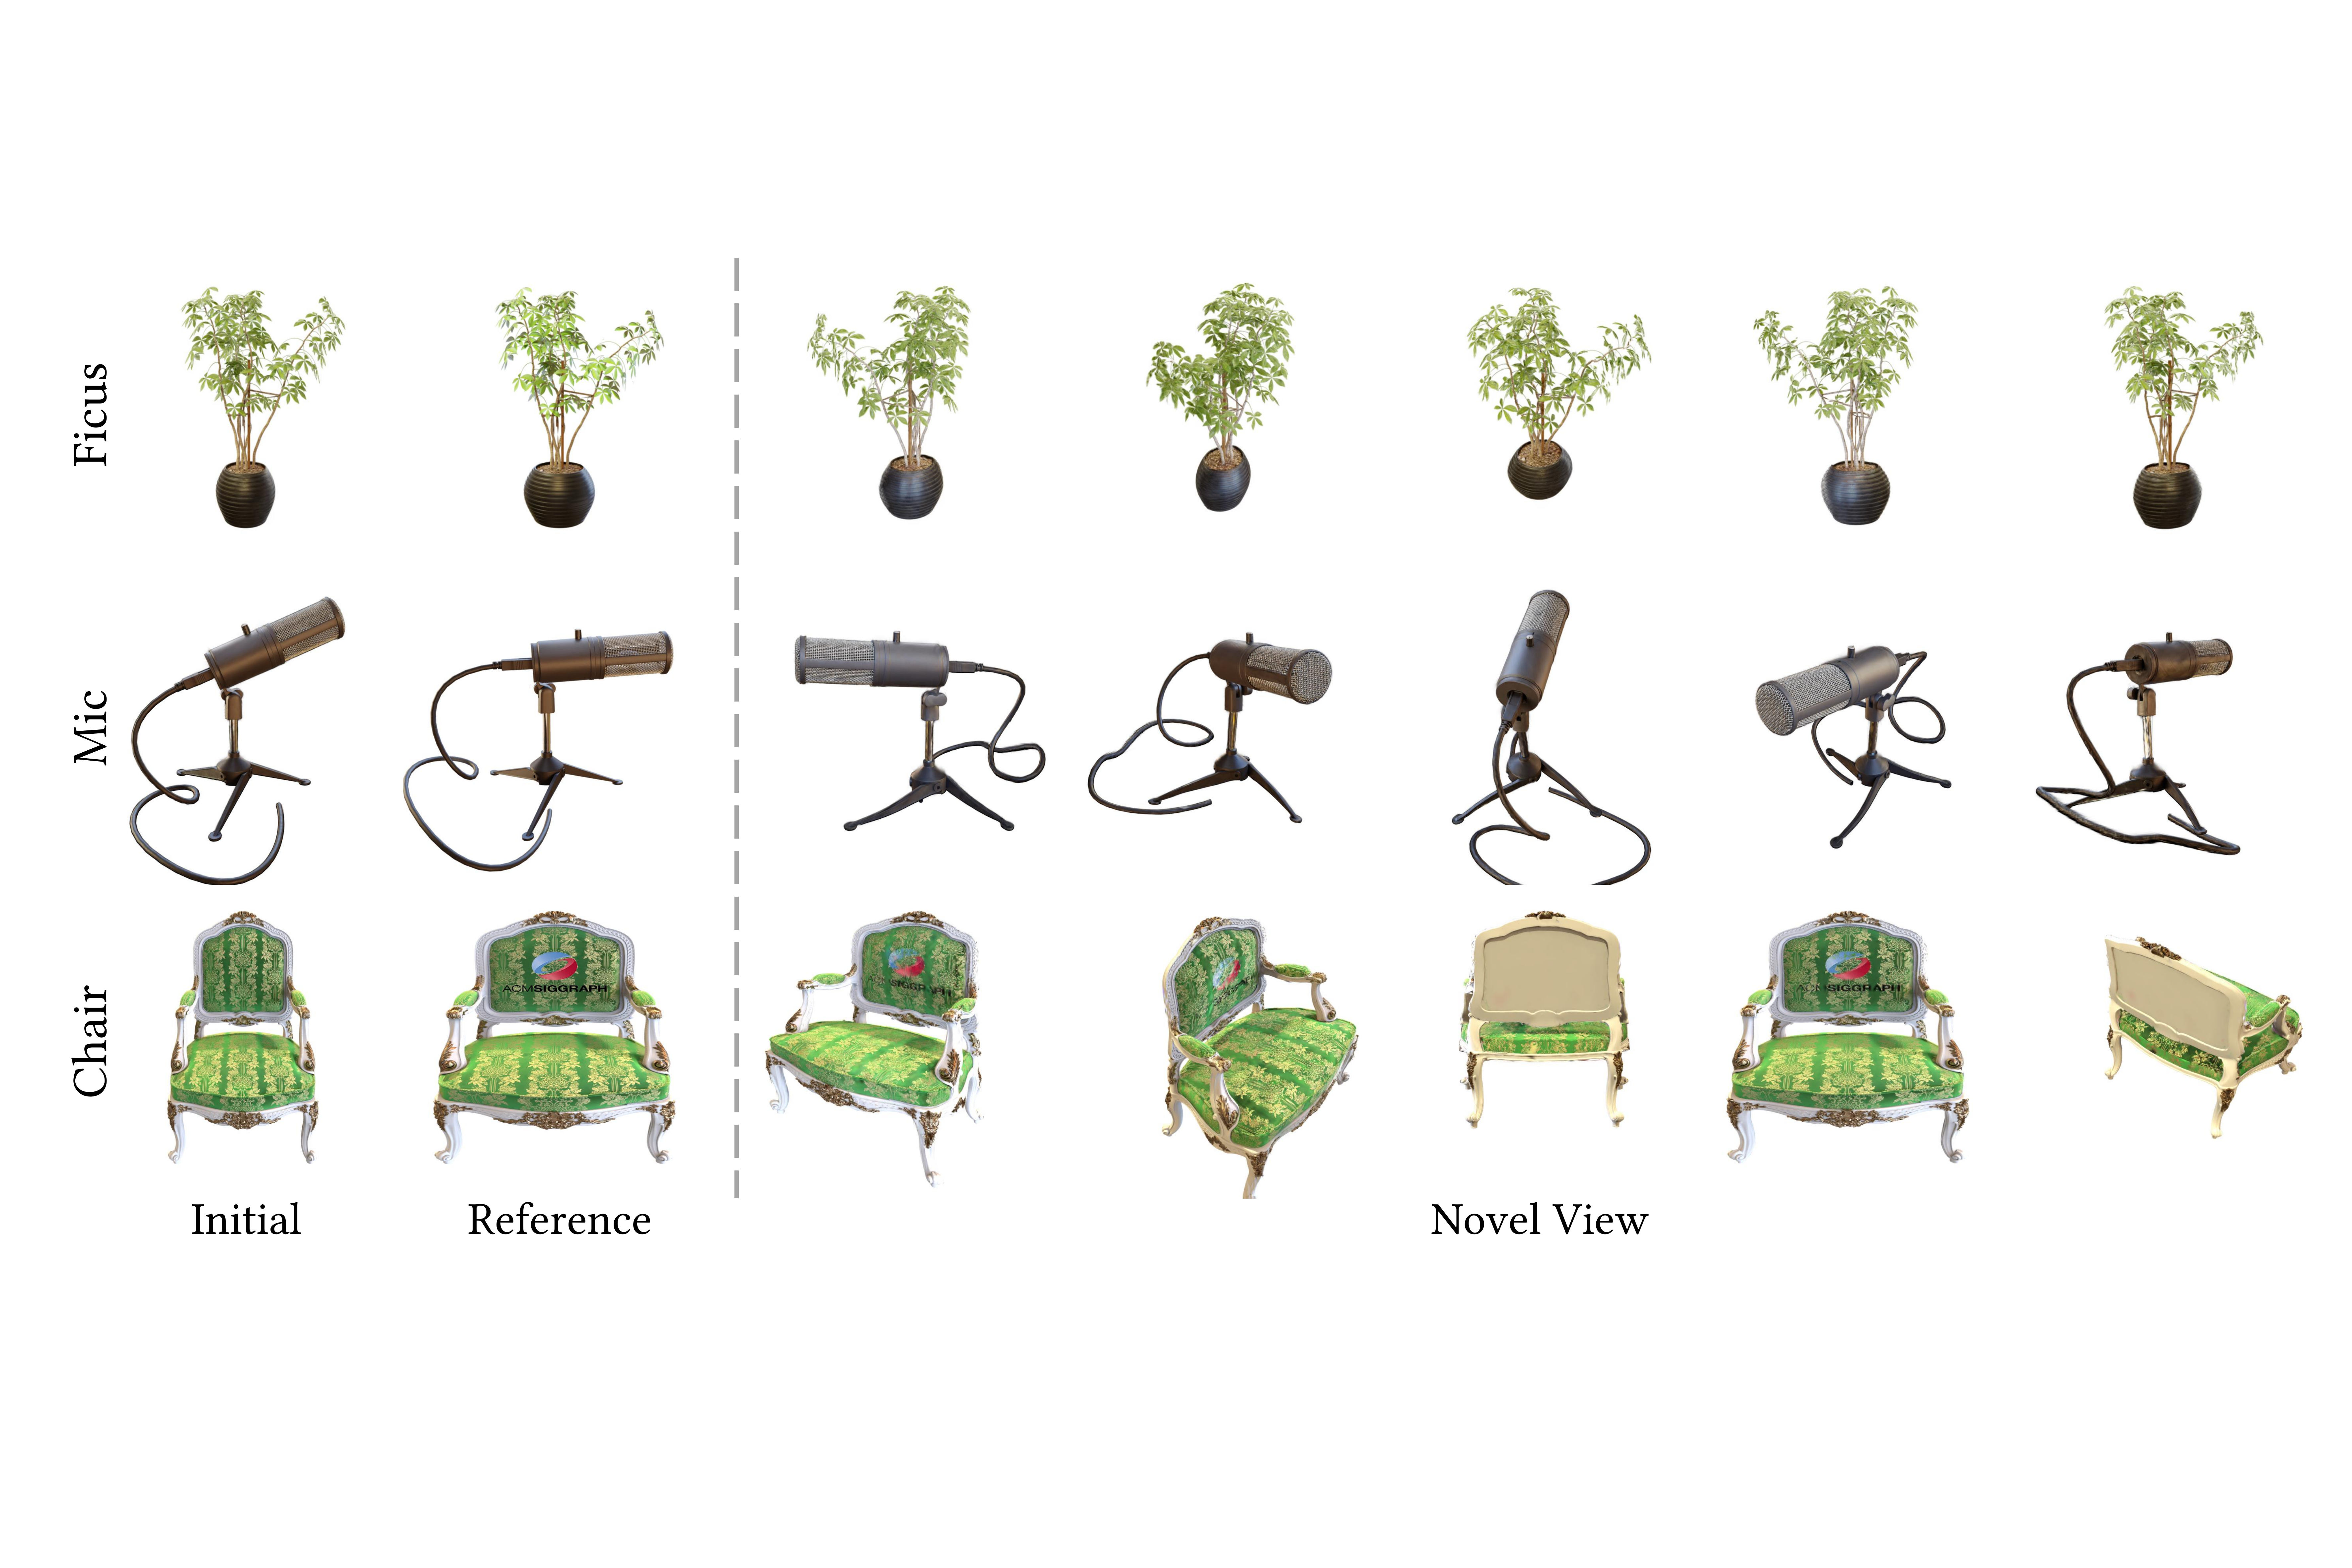}
    \caption{\textbf{Novel view results on NS dataset.} }
    \label{fig:appendix-nvs-nerf}
\end{figure*}
